# Supplementary material for: TranSQL+: Serving Large Language Models with SQL on Low-Resource Hardware
Source: arXiv:2502.02818 source file (2025-09-21)
Supplement: Supplementary file 1 [file appendix.tex]

\appendix
\section{Additional Templates}
\label{app:A}
\subsection{Primary Categories}
\para{Element-wise Arithmetic}
Element-wise arithmetic operations involve two matrices performing addition or multiplication on a per-element basis. Since the operation is applied independently to each corresponding element, all dimensions must be exactly aligned between operands—thus, all dimensions are considered \emph{shared dimensions}.

Taking element-wise addition as an example, let $X = A + B$ where $A, B \in \mathbb{R}^{m \times n}$. The computation is defined as:
\[
x_{ij} = a_{ij} + b_{ij}, \quad \text{for } i \in [0, m),\ j \in [0, n).
\]
This can be parameterized as:
\[
\operatorname{ADD}\Bigl(\{A, B\},\, \varnothing,\, \{(m_A, m_B),\ (n_A, n_B)\},\,\varnothing\Bigr),
\]
where $\varnothing$ indicates no free dimensions, and each pair in the shared dimension set denotes the dimension alignment between operands $A$ and $B$.

\para{Reshape}
Shape manipulation is a common class of operations in large language models, often used to flatten, split, or permute dimensions to match the expected shape for subsequent computations. These transformations do not change the underlying data but reorganize its dimensional structure.

As an example, consider a reshape operation that flattens two adjacent dimensions. Suppose tensor $A \in \mathbb{R}^{m \times n \times p}$ is reshaped to $B \in \mathbb{R}^{m \times q}$, where $q = n \cdot p$. The merging rule—i.e., which dimensions to combine and how—is an operator-specific attribute.

We parameterize this reshape operation as:
\[
\operatorname{Reshape}_{(n,\,p) \rightarrow (n \cdot p)}\bigl(\{A\},\, \varnothing,\, \{m\},\, \{(n, p)\}\bigr).
\]
Here, the dimension $m$ is treated as a shared dimension because, under SQL semantics, the reshape can be interpreted as an operation over two columns derived from a self-join on the input relation. However, in practice, the self-join can be bypassed, and the transformation can be applied directly on the relevant columns using projection logic. This simplification avoids unnecessary overhead during query execution.

The transformation rules are represented as lambda functions (e.g., $(n, p) \mapsto n \cdot p$), which can be directly implemented using projection expressions in the corresponding SQL templates. Similarly, a dimension permutation such as swapping axes can be expressed with an attribute like $(n, p) \mapsto (p, n)$, which is also resolved at the projection step.

\subsection{Special Case}
\para{Slice and Concat} Another group of special operators includes \texttt{slice} and \texttt{concat}. Unlike the core categories, which typically produce a single result chunk or scalar, these operators alter the chunk structure of the relation. The \texttt{slice} operator produces new chunks that are parallel to the original ones in the same relation, representing logical partitioning along a specified dimension. In contrast, \texttt{concat} merges multiple chunks into a single one along a specified axis. Both operations are performed within the same relational table and maintain dimensional consistency but modify the layout of the data across chunks.
